# Supplementary material for: Testing Symmetric Markov Chains from a Single Trajectory
Source: arXiv:1704.06850 source file (2017-12-04)
Supplement: Supplementary file 5 [file appendix_riffle_lb.tex]

In this section we will show that any algorithm that tests identity of a sparse Markov chain representing 
card riffle shuffling requires at least $\Omega\left({\frac{n}{\eps^2}}\right)$ independent trials, where 
each trial is a $n$-length word generated by a sparse Markov chain.
We recall Definition~\ref{def:sparse} of a sparse Markov chain adapting it slightly for the convenience of lower bound presentation.
Sparse Markov chains $P=\{P_t\}_{t=1}^{T}, Q=\{Q_t\}_{t=1}^{T}$: each independent run consists of $T=O(n)$ time steps; has $O(n)$ states for each time $t$;  Markov chain starts
from a single state at $t=0$ ; there are only $O(1)$ possible transitions $P_t(ij)\neq 0$ from each state 
$i$ to other states for all but the very first time step $t>0$. 

\begin{theorem}[Sparse Lower Bound]
\label{thm_app:sparse-lower-bound}
There is an instance of Identity testing problem for a sparse Markov chain $Q$ that requires
at least $m\ge\Omega(\frac{n}{\eps^2})$ i.i.d. samples to check identity of $Q$ with $99$\% confidence\footnote{We assume
$\eps=\omega(n^{-1/6})$ in the requirement $\dist{P}{Q}\ge\eps$, when $P\neq Q$.}.
%There exists a constant $c>0$, such that any algorithm which, given the description of a sparse Markov chain $Q$ with 
%$O(n)$ layers and each layer containing $O(n)$ states, and sample access to words from another sparse Markov chain $P$ 
%over the same set of states as $Q$, distinguishes between the cases $P \equiv Q$ and $\dist{P}{Q} \ge \eps$ with 
%probability at least $99/100$ requires at least $k \geq \frac{cn}{\eps^2}$ samples.
\end{theorem}
\begin{proof}
The high-level proof idea is similar to that of Theorem~\ref{thm_app:symm-lower-bound}. At an abstract level, we construct a sparse Markov chain $Q$, 
with respect to which we are interested in testing identity, and a class of sparse Markov chains $\mathcal{P}$ such that 
\begin{enumerate}
%\item $\mathcal{Q}$ is a single Markov chain $Q$ which identity we are testing. 
\item Every $P \in \mathcal{P}$ is at least $\eps$ far from $Q$, i.e., $\dtv{\word{P}{T}}{\word{Q}{T}}\ge \eps$ for any $P \in \mathcal{P}$.
\item There is a constant $c > 0$, such that it is impossible to distinguish $m$ i.i.d. samples of $T$-length words generated by 
a random Markov chain $\bar{P}\sim \mathcal{P}$ from the samples produced by $Q$ with probability 
equal to or greater than $\frac{99}{100}$, for $m\le\frac{cn}{\eps^2}$.
\end{enumerate}

We denote the joint distribution of $m$ i.i.d. samples from $Q$ by $Q^{\otimes m}$ and that from $\bar{P}$ by $\bar{P}^{\otimes m}$.
To prove the last point we show that $\dtv{Q^{\otimes m}}{\bar{P}^{\otimes m}}$ is small for some $m=\Om{\frac{n}{\eps^2}}$.
We now describe our construction. To simplify presentation, we use multi-edges in the description of sparse Markov chains.
We convert this instance into simple edge graph by the same duplicating trick we employed in 
the lower bound construction of Theorem~\ref{thm_app:symm-lower-bound}.

%We respectively denote the words of length $m$ obtained from $Q$ by $\word{Q}{m}$, and from a Markov chain $\bar{P}\sim\mathcal{P}$ by $\word{\bar{P}}{m}$.\\
%We will assume $n$ is odd without loss of generality for the following lower bound construction.
%\noindent 

\begin{description}
\item[Markov Chain $Q$:] $T=2n+1$ time steps; single state at $t=0$, states $[2n]$ at each $1\le t\le T$.
All states are divided into two categories: {\em Frequently} visited ($F$) $\eqdef\{2i-1, i\in[n]\}$ and {\em Rare} ($R$) $\eqdef\{2i,i\in[n]\}$.
Table below describes weighted multi-graph $Q=\{Q_t\}_{t=1}^{T}$: $x\in F,$ $y\in R$, $x,y\in [2n]$ denote respective generic frequent and rare states. 
We adopt notational convention: $0\eqdef 2n$, $2n+1\eqdef 1$.   

\begin{tabular}{r|c|c|c|c}
        &  $F\to F$        & $F\to R$       & $R\to F$       &     $R\to R$   \\ 
%				&  $(2i\to 2j)$    & $(2i\to 2j+1)$ & $(2i+1\to 2j)$ & $(2i+1\to 2j+1)$ \\ 
\hline
\multicolumn{1}{ r| }{\multirow{2}{*}{t=1:} }
        &  $(1\to x)\in E$                  & \multicolumn{1}{|c|}{\multirow{2}{*}{$\emptyset$}} &  \multicolumn{1}{|c|}{\multirow{2}{*}{$\emptyset$}} 
				                                                                                     & \multicolumn{1}{|c}{\multirow{2}{*}{$\emptyset$}}                  \\ %\hline
				& $Q_{1}(1,x)=\frac{1}{n}$       &                                                   &                                                     &              \\ \hline
\multicolumn{1}{ r| }{\multirow{2}{*}{t=2k:} }
        & $(x\to x)\in E$             &  $(x\to x\pm 1)\in E$           &  $(y\to y\pm 1)\in E$           & \multicolumn{1}{|c}{\multirow{2}{*}{$\emptyset$}}     \\ %\hline
        & $Q_t(x,x)=1-\frac{2}{n}$ &  $Q_t(x,x\pm 1)=\frac{1}{n}$ &  $Q_t(y,y\pm 1)=\frac{1}{2}$ &                                                       \\ \hline
\multicolumn{1}{ r| }{\multirow{2}{*}{t=2k+1:} }				
        &  $(x\to x)\in E$            &  \multicolumn{1}{|c|}{\multirow{2}{*}{$\emptyset$}} &  \multicolumn{1}{|c|}{\multirow{2}{*}{$\emptyset$}} 
				                                                                                       &  $(y\to y)_{1,2}\in E$                               \\ %\hline
        &  $Q_t(x,x)=1$            &                                                     &                                                     
				                                                                                       &  $Q_t(e_1)=Q_t(e_2)=\frac{1}{2}$                                  \\ %\hline
\end{tabular}
%\begin{align*}
%t=1:& \quad\quad \forall 2i+1\in[2n]\quad \quad (1,2i+1)\in E\quad  \quad Q_{1}(1\to 2i+1)=\frac{1}{n}\\
%t=2k:& \quad\quad \forall i\in[2n]\quad \quad (1i)\in E\quad  \quad Q_{1}(1i)=\frac{1}{2n}\\
%t=2k+1:& \quad\quad \forall i\in[2n]\quad \quad (1i)\in E\quad  \quad Q_{1}(1i)=\frac{1}{2n}
%%Q_{(ij)_1}=\frac{1}{2(n-1)} \quad\quad Q_{(ij)_2}=\frac{1}{2(n-1)}\quad\quad \text{ for any } i\neq j.
%\end{align*}
\item[Family $\mathcal{P}$:] every $P \in \mathcal{P}$ has the same set of states and edges as $Q$.
Similar to the construction in Section~\ref{sec:symmetric_lb}, we only change weights of the multi-edge 
pairs (independently and uniformly at random for each pair $(y\to y)_{1,2}$ and time $t$): 
\[
P_{t}(e_{1,2})=\frac{1\pm 4\eps}{2} \quad\quad\text{ or }\quad\quad
P_{t}(e_{1,2})=\frac{1\mp 4\eps}{2}.
\]
\end{description}

The idea of this construction is that a typical trajectory of Markov chain $Q$ or $P\in\mathcal{P}$ 
stays in frequent states almost all the time and very rarely visits one of the rare states.  However,
a typical trajectory has constant probability of visiting a rare state.
\begin{lemma}
\label{clm:p-far-from-q shuffle}
Any $P \in \mathcal{P}$ is at least $\eps$-far from $Q$, i.e., $\dist{P}{Q}= \dtv{\word{P}{T}}{\word{Q}{T}}\ge\eps$.
\end{lemma}
\begin{proof}
Consider a $P \in \mathcal{P}$. First, we argue that probability of any word $w$
with only a single visit to a rare state (at even $t=2k$) satisfies $\left| \Prx[Q]{w} - \Prx[P]{w}\right|  = 4\eps\cdot\Prx[Q]{w}.$
%We will show $\dist{P}{Q}$ is large by arguing that the probability of any word 
%with only one visit to a rare state at even time step $t=2k$ differs under $Q$ and under $P$ by at least $2\eps$ factor. 
Indeed, let visit to the rare state $2i$ in $w$ happen at the time $t=2k$, then
\[
\begin{cases}
\Prx[Q]{w} = \Prx[Q]{s_1 \ldots s_{2k}}\cdot \frac{1}{2} \cdot \Prx[Q]{s_{2k+1} \ldots s_{2n+1}|s_{2k+1}}\\
\Prx[P]{w} = \Prx[P]{s_1 \ldots s_{2k}}\cdot \frac{1}{2}(1 \pm 4\eps) \cdot \Prx[P]{s_{2k+1} \ldots s_{2n+1}|s_{2k+1}}.
\end{cases}
\]
Therefore, as $Q$ and $P$ have the same transitional probabilities of $s_t\to s_{t+1}$ for $t\neq 2k$, we get 
$$\left| \Prx[Q]{w} - \Prx[P]{w}\right|  = 4\eps\cdot\Prx[Q]{w}.$$ 
Now, the probability of visiting a rare state exactly once (at even $t$) in $Q$ is precisely 
\[
\sum_{\substack{w \text{ with}\\ \text{1 rare visit}}} \Prx[Q]{w} = n\cdot\frac{2}{n}\cdot\left(1-\frac{2}{n}\right)^{n-1}> 2\cdot e^{-2}>\frac{1}{4},
\]
where we used inequality $(1-\frac{1}{n})^{n-1}> e^{-1}$ to get the estimate in the right hand side.
%The probability of 0 visits to rare states is $(1-2/n)^{n} \le e^{-4}$. Conditioned on there being a visit to a 
%rare state, the probability of 0 additional visits to rare states in even-indexed layers is $(1-2/n)^{2n-2} \le 
%4e^{-4}$ for $n \ge 4$. Hence the probability of exactly one rare state visit in an even-indexed layer is 
%$\ge (1-e^{-4})(1-4e^{-4}) \ge 1/2$. 
Hence, 
\begin{align*}
\dtv{\word{P}{T}}{\word{Q}{T}} \ge \sum_{\substack{w \text{ with}\\ \text{1 rare visit}}} 
\left|\Prx[Q]{w} - \Prx[P]{w}  \right| =  \sum_{\substack{w \text{ with}\\ \text{1 rare visit}}}4\eps\cdot\Prx[Q]{w} 
\ge 4\eps\cdot\frac{1}{4} = \eps.
\end{align*}
%From the relation between total variation and Hellinger squared distances and Claim \ref{clm:dist-monotone}, we 
%have that, $\dist{P}{Q} \ge \hellingersq{P}{Q} \ge \hellingersq{P}{Q}_2$. Under our construction, $\oneet \circ 
%\srprod{P_1}{Q_1} = \frac{1}{n}\onev^{\text{T}}$ and it can be seen that $\oneet \circ \srprod{P_1}{Q_1} \circ 
%\srprod{P_2}{Q_2} \circ \onev \le 1-\eps$. Hence $\hellingersq{P}{Q}_2 \ge \eps$ thereby proving the claim.
\end{proof}

%We group transitions within a single word into two categories: Those which occur from a frequent state and those 
%which occur from a rare state. Note that from a rare state, the transition has to happen to a frequent state. 
We define collisions and $3$-way collisions similar to the proof of Theorem~\ref{thm_app:symm-lower-bound}. Namely,
a collision is a transition that occurs in two samples (3-way collision -- in at least three samples) of $Q^{\otimes m}$ or $P^{\otimes m}$ from the 
same state and at the same time. Moreover, as $P\sim\mathcal{P}$ and $Q$ are the same except for the double edges
between rare states, we are only interested in the collisions along multi-edges between rare states. 
%If the same transition repeats in two samples, we call it a collision. If it occurs in 3 distinct samples, we 
%call it a 3-way collision. We make the following observations about $Q$ and $\mathcal{P}$.

\begin{lemma}
\label{clm:num-collisions shuffle}
The expected number of collisions in samples $Q^{\otimes m}$ is $O\left(\frac{m^2}{n^2} \right) = O\left(\frac{1}{\eps^4} \right)$.
%Consider a sample from $Q^{\otimes m}$. The expected number of collisions among transitions from a rare state 
%to another rare state is $O\left(\frac{m^2}{n^2} \right) = O\left(\frac{1}{\eps^4} \right)$.
\end{lemma}
\begin{proof}
Let $I_w(m_1,m_2,y,t)$ indicate the event that either of the transitions along edges $e_{1,2}=y\to y$ at time $t$, occurred in samples $m_1$ and $m_2$. 
Note that at each fixed time all of the $n$ frequent states are equally likely to occur in a sample from $Q$. Therefore, the probability of visiting given
rare state $y$ at time $t$ in a single run is at most $O(1/n^2)$. 
%probability is uniformly spread over all $n$ frequent states and the probability of 
%transitioning to a rare state from a frequent state is $2/n$.
This implies 
$\Prx[Q]{I_w(m_1,m_2,y,t) = 1} = O\left(\frac{1}{n^2}\cdot \frac{1}{n^2}\right) = 
O(1/n^4)$.
%because at each time probability is uniformly spread over all $O(n)$ frequent states and the probability of 
%transitioning to a rare state from a frequent state is $2/n$. 
Let $X$ denote the total number of collisions.
\begin{align*}
\Ex{X} &= \sum_{m_1 \neq m_2}\sum_{i\neq j} \Ex{I_w(m_1,m_2,y,t)} = O\left(m^2n^2 \frac{1}{n^4} \right) = 
O\left(\frac{m^2}{n^2} \right)
\end{align*}
\end{proof}

\begin{lemma}
\label{clm:3-way collision shuffle}
The probability of a 3-way collision in samples $Q^{\otimes m}$ is $o(1)$.
%Consider $m=\frac{n}{\eps^2}$ samples from either $Q$. The probability of a 3-way collision 
%among the $m$ samples is $o(1)$.
\end{lemma}
\begin{proof}
Similar to the proof of Lemma~\ref{clm:num-collisions shuffle} we can give an upper bound on the expected number of 
$3$-way collisions being $\Ocomplex{n^2m^3\cdot\frac{1}{n^6}\cdot }=\Ocomplex{\frac{m^3}{n^4}}$. Markov's inequality concludes 
the proof.
\end{proof}

Now consider a typical set of $m$ words generated by $Q$ (or equivalently drawn from $Q^{\otimes m}$).
%$\bar{P}\sim\mathcal{P}$. 
As we know from Lemma~\ref{clm:3-way collision shuffle} it has no 3-way collisions and by Markov's inequality 
and Lemma~\ref{clm:num-collisions shuffle} has at most $O(\frac{1}{\eps^2})$ collisions with probability greater 
than $9/10$ (for sufficiently small $c>0$ and $m=\frac{cn}{\eps^2}$). As we show next a typical set of $m$ words drawn from 
$Q$ has similar probability under the $\bar{P}\sim\mathcal{P}$ and $Q$ models.

\begin{lemma}
\label{clm:no-collision-analysis shuffle}
At least $1/2$ of the sets $S = \{w_1,\ldots,w_m\}$ of samples from $Q^{\otimes m}$ satisfy 
$$ \frac{1}{2}\cdot\prob[Q^{\otimes m}]{S}<\prob[\bar{P}^{\otimes m}]{S} < 2\cdot \prob[Q^{\otimes m}]{S}$$
\end{lemma}
\begin{proof}
We consider the ratio of the respective probabilities $(*)\eqdef\frac{\prob[\bar{P}^{\otimes m}]{S}}{\prob[Q^{\otimes m}]{S}}$. As in 
Lemma~\ref{clm:no-collision-analysis}, both probabilities in the numerator and denominator can be expressed in terms of 
simple statistics for the set $S$, specifically the number of single step transitions between pairs of states. 
Also similar to the Lemma~\ref{clm:no-collision-analysis}, the corresponding multiplicative terms for $\bar{P}^{\otimes m}$ 
and $Q^{\otimes m}$ are identical except for the collisions along multi-edges between two rare states (at least two transitions between
a pair of rare states). Moreover, we also differentiate type I and type II collisions between rare states: (type I) transitions between
rare states $y\to y$ at time $t$ were made along different edges $e_1$ and $e_2$; (type II) two transitions were made along the same edge
either $e_1$, or $e_2$. Per type I and II collisions the corresponding terms in $(*)$ are respectively
$(1-4\eps)(1+4\eps)=1-16\eps^2$ and $1+16\eps^2$.

We further continue following the proof of the Lemma~\ref{clm:no-collision-analysis}, and make sure that with high probability there are only $X=O(\frac{1}{\eps^4})$ collisions and
no $3$-way collisions in $S$. We can make sure that the difference between numbers of type I and type II collisions is at most $O(\sqrt{X})=O(\frac{1}{\eps^2})$ 
with probability at least $3/4$, as the choice of collision type in $w$ under $Q$ model is uniform between type I and type II and independent across different collisions.
For small enough $m=\Omega(\frac{n}{\eps^2})$ we can make sure that at least $\frac{1}{2}$ fraction of words $w$ under $Q$ model have the number of collisions
at most $\frac{c_1}{\eps^4}$ and also have the difference between number of type I and type II collisions at most $\frac{c_2}{\eps^2}$, for some small constants $c_1,c_2>0$.
In this case we get the following bounds on $(*)$.
\[
2>\left(1+16\eps^2\right)^{\frac{c_2}{\eps^2}}>\frac{\prob[\bar{P}^{\otimes m}]{S}}{\prob[Q^{\otimes m}]{S}}>
\left(1-256\eps^4\right)^{\frac{c_1}{2\eps^4}}\cdot \left(1-16\eps^2\right)^{\frac{c_2}{\eps^2}}>1/2
\]

\end{proof}

Lemma~\ref{clm:no-collision-analysis shuffle} shows that $\dtv{Q^{\otimes m}}{\bar{P}^{\otimes m}} \leq \frac{3}{4}$ for $m 
\leq \frac{cn}{\eps^2}$ for some constant $c$, which implies that no algorithm can successfully distinguish $Q$ from the family 
$\mathcal{P}$ with probability greater than $\frac{3}{4}$ for some $m=\Omega(\frac{n}{\eps^2})$.
\end{proof}
