# Supplementary material for: Testing Symmetric Markov Chains from a Single Trajectory
Source: arXiv:1704.06850 source file (2017-12-04)
Supplement: Supplementary file 6 [file appendix_riffle_ub.tex]

We consider all one-step transitions that can have positive probability in the Markov chain $Q$ or $P$, we call these one-step transitions as {\em edges}. 
We denote a generic edge from a state $s_{i,t-1}$ to a state $s_{j,t}$ by $e$; the set of all possible edges by $E$; the set of transitions in $E$ between 
states at time $t-1$ and time $t$ by $E(t)$ for each $t\in[n]$. 
%We also add new edges $E(0)$ to $E$, which indicate transitions to the original states at 
%time $t=0$ with positive probabilities in $q_0$ or $p_0$. 
For each edge $e$, let $q_e$ and $p_e$ be the probabilities that there was a transition along 
edge $e$ in one sample $s_1\cdots s_n$ from $Q$, or from $P$, respectively.
Our test, from a high level perspective, consists of two steps: 
\begin{description}
 \item[Pruning.] We remove all {\em rare edges}, i.e., edges that are traversed with probability less than $O(\frac{\eps^2}{n^2})$ in $Q$. Let $E^*$ be 
the resulting pruned set of edges. We reject all samples from $P$ that go along any removed edge $e\notin E^*$. We return $P\neq Q$ if there are too many 
rejected samples. Otherwise, we continue to the next step.
 \item[$\chi^2$-statistic on edges.] For each non rare edge $e\in E^*$ we count the number of transitions $n_e$ along $e$. We define $\chi^2$ 
{\em edge statistic} $Z_e\eqdef\frac{(n_e-q_e\cdot m)^2-n_e}{q_e\cdot m}$. Our main statistic is 
  \[
      Z\eqdef\sum_{e\in E^*}Z_e =\sum_{e\in E^*}\frac{(n_e-q_e\cdot m)^2-n_e}{q_e\cdot m}.
  \]
  We accept or reject $P=Q$ depending on $Z$ being smaller or larger than a certain threshold.
\end{description}
In the remainder of this section we mostly focus on the latter step. Specifically, we analyze the $\chi^2$ edge statistic in the case when 
$q_e\ge\Omega(\frac{\eps^2}{n^2})$ for all $e\in E$ and $p_e=0$ for all $e\notin E$. At the end of the section we explain why after the pruning step these conditions 
are satisfied. 

%Poisson number of samples with expectation $m$.
\paragraph{Poisson Sampling.} Throughout the analysis of $\chi^2$ statistic, we use the standard Poissonization approach. 
Instead of drawing exactly $m$ samples from $P$, we first draw $m'\sim\Poisson{m}$, and then draw $m'$ samples from $P$. 
The benefit of this is that the number of times different elements in the support of the cut distribution occur in the sample become 
independent, giving simpler analysis. Moreover, the number of transitions observed along the edge 
$e\in E(t)$, $n_e$, for a fixed $t$ will be distributed as $\Poisson{m\cdot p_e}$, independently for all $e\in E(t)$ (see Lemma~\ref{cl:ind_poisson}). As 
$\Poisson{m}$ is tightly concentrated around $m$, this additional flexibility comes only at a sub-constant cost in 
the sample complexity with an inversely exponential in $m$, additive increase in the error probability. We note that 
as in equations $(1-2)$ from~\cite{AcharyaDK15} the expectation and variance of our $\chi^2$ statistic are as follows.
\[
\Ex{Z_e}=m\cdot\frac{(p_e-q_e)^2}{q_e} 
\quad\text{and}\quad 
\Var{Z_e}=2\frac{p_e^2}{q_e^2}+m\cdot\frac{p_e(p_e-q_e)^2}{q_e^2}.
\]

\begin{lemma}
 \label{cl:ind_poisson}
The number of transitions $n_e$ along an edge $e$ is distributed as $\Poisson{m\cdot p_e}$ and all $n_e$ are independent for $e\in E(t)$, for any
$t\in[n]$.
\end{lemma}
\begin{proof}
The proof proceeds by induction on $t$ and is based on the following two standard observations on Poisson random variables:

\textit{(Observation I)} for any discrete distribution $\distr$, $k\sim\Poisson{\lambda}$ i.i.d. samples from
$\distr$ form a collection of jointly independent Poisson random variables for the occurrences of each element in 
the support of $\distr$, i.e., distribution $\prod_i\Poisson{\lambda\cdot\Prx[x\sim\distr]{x=i}}$;

\textit{(Observation II)} the sum of two independent Poisson random variables with distributions $\Poisson{\lambda_1}$ and $\Poisson{\lambda_2}$
is a Poisson random variable with the distribution $\Poisson{\lambda_1+\lambda_2}$.

For $t=1$ as we start with $\Poisson{m}$ samples,  Observation I gives us the desired result. For the induction step (from $t=k$ to $t=k+1$), we observe that counts of visits to each particular state $i$ at time $t$ are independent Poisson random variables by Observation II. Now, Observation I 
applied to the states at time $t$ yields the desired result.
\end{proof}

The following procedure correctly distinguishes between the case $P=Q$, or $\dist{P}{Q}\ge\eps$, in the regime when $q_e\ge\Omega(\frac{\eps^2}{n^2})$ 
for all $e\in E(Q)$ and $p_e=0$ for all $e\notin E$.

\begin{algorithm}[H]
\caption{$\chi^2$ Edge Test}
\label{alg:chi_sq_edges}
\KwIn{$\eps$; an explicit $k$-sparse Markov Chain $Q=\MCseqQ$; (Poisson) $m$ samples from a Markov Chain $P=\MCseqP$, where $n_e$ 
denotes the number of transitions along the edge $e$.}
\KwOut{Accept if $P=Q$, or reject if $\dist{P}{Q}\ge\eps$}
\BlankLine
$E\leftarrow\{e: q_e> 0\}$\;  
$Z\leftarrow\sum\limits_{e\in E} \frac{(n_e-q_e\cdot m)^2-n_e}{q_e\cdot m}$\; 
%\eIf{$Z\le\frac{\eps\cdot m}{4}$}
\eIf{$Z\le 2\sqrt{k}n^{3/2}$}
{
\KwRet \textsc{Accept}\;  
}
{
\KwRet \textsc{Reject}\;  
}
\end{algorithm}

\begin{theorem} 
Algorithm~\ref{alg:chi_sq_edges} is correct with probability at least $4/5$, if $m\ge\frac{C n^{3/2}}{\eps^2}$ for some $C=O(1)$, 
$q_e\ge\frac{\eps^2}{kn^2}$ for all $e\in E$, and $p_e=0$ for all $e\notin E$.
\label{th:sparse_ub}
\end{theorem}
\begin{proof} To get the desired result we analyze expectation and variance of $Z$. First, we relate the expected value of $Z$ with the distance $\dist{P}{Q}$ between $P$ and $Q$.

\begin{lemma}
\label{cl:expectation_dist}
%%$\Ex{Z}\ge m\cdot\hellingersq{P}{Q}.$
$\Ex{Z}\ge \frac{m}{4}\cdot\distsq{P}{Q}.$
\end{lemma}
\begin{proof}
We recall that 
\begin{multline}
\label{eq:dist_P_Q_sum}
\hellingersq{P}{Q}  =1-\oneet\circ\srprod{P_1}{Q_1}\circ\cdots\circ\srprod{P_t}{Q_t}\circ\cdots\srprod{P_n}{Q_n}\circ\onev\\
 = \oneet\circ\left(\frac{P_1+Q_1}{2}\right)\circ\cdots\circ\left(\frac{P_n+Q_n}{2}\right)\circ\onev-
   \oneet\circ\srprod{P_1}{Q_1}\circ\cdots\srprod{P_n}{Q_n}\circ\onev\\
 =\sum_{t=1}^{n} \oneet\circ\srprod{P_1}{Q_1}\circ\cdots\circ\left(\frac{P_t+Q_t}{2}-\srprod{P_t}{Q_t}\right)\circ\left(\frac{P_{t+1}+Q_{t+1}}{2}\right)\cdots
\left(\frac{P_{n}+Q_{n}}{2}\right)\circ\onev\\
=\frac{1}{2}\sum_{t=1}^{n} \oneet\circ\srprod{P_1}{Q_1}\circ\cdots\circ\srprod{P_{t-1}}{Q_{t-1}}\circ\sqsrprod{P_t}{Q_t}\circ\onev,
\end{multline}
where in the last line $\sqsrprod{P_t}{Q_t}=\left(\left(\sqrt{P_t(ij)}-\sqrt{Q_t(ij)}\right)^2\right)_{ij}$. Indeed, the first equality holds true as
$P_t\circ\onev=Q_t\circ\onev=\onev$ for any $t\in[n]$; the second equality is a telescopic sum; the last equality is simply the formula for the complete square. 
Let $q_t$ and $p_t$ be the respective distribution vectors over the states $s_{i,t}$, $i\in[n]$ in $Q$ and $P$ Markov chains. We also define distributions $p_0=q_0=\onee$.

By applying Cauchy-Schwarz inequality to the corresponding Bhattacharya coefficient of $P$ and $Q$ at a fixed state $i$ and time $t$  
we obtain
\begin{align*}
\oneet\circ\srprod{P_1}{Q_1}\circ\cdots\circ\srprod{P_{t}}{Q_{t}}\circ\onevi=
HS_i\left(\word{P}{t},\word{Q}{t}\right)  = \sum_{\substack{w=s_0\ldots s_t \\ \text{s.t. } s_t=i}}  \sqrt{\Prl[P]{w}\Prl[Q]{w}}\\
\le\sqrt{\sum_{\substack{w=s_1\ldots s_t \\ \text{s.t. } s_t=i}}  \Prl[P]{w}\sum_{\substack{w=s_1\ldots s_t \\ \text{s.t. } s_t=i}}\Prl[Q]{w}} 
=\sqrt{p_t(i)\cdot q_t(i)}.
\end{align*}
We plug in this estimate to \eqref{eq:dist_P_Q_sum} and obtain
\[
\frac{1}{4}\cdot\distsq{P}{Q}=\frac{1}{4}\dtvsq{P}{Q}\le \hellingersq{P}{Q}  \le \frac{1}{2}\sum_{t=1}^{n} \srprodt{p_{t-1}}{q_{t-1}}\circ\sqsrprod{P_t}{Q_t}\circ\onev,
\]
%where $p_{-1}=q_{-1}$ is a probability distribution with one element in the support and $P_0$ and $Q_0$ are the $1\times n$ matrices corresponding to $p_0$ and $q_0$ vectors. 
We examine each term of the summation in the right hand side of the last equation
\be
\label{eq:dist_sqrtpq}
\frac{1}{2}\srprodt{p_{t-1}}{q_{t-1}}\circ\sqsrprod{P_t}{Q_t}\circ\onev=\sum_{i}\frac{\sqrt{p_{t-1}(i)\cdot q_{t-1}(i)}}{2}\cdot\sum_{j:(ij)\in E(t)}
\left(\sqrt{P_t(ij)}-\sqrt{Q_t(ij)}\right)^2,
\ee
We show that corresponding terms in $\Ex{Z}=\sum\limits_{i,t}\sum\limits_{e:(ij)\in E(t)}\Ex{Z_e}$ give an upper bound on \eqref{eq:dist_sqrtpq} for each fixed state $i$.

\begin{multline}
\frac{1}{m}\sum_{e:(ij)\in E(t)}\Ex{Z_e}=\sum_{e:(ij)\in E(t)}\frac{(p_e-q_e)^2}{q_e}=\sum_{j:(ij)\in E(t)}
\frac{\left(p_{t-1}(i)P_t(ij)-q_{t-1}(i)Q_t(ij)\right)^2}{q_{t-1}(i)Q_t(ij)}\\
%=\frac{p_{t-1}^2(i)}{q_{t-1}(i)}\sum_{j:(ij)\in E(t)}\frac{P_t^2(ij)}{Q_t(ij)}-2p_{t-1}(i)\sum_{j:(ij)\in E(t)}P_t(ij)+q_{t-1}(i)\sum_{j:(ij)\in E(t)}Q_t(ij)\\
=\frac{p_{t-1}^2(i)}{q_{t-1}(i)}\left(\sum_{j:(ij)\in E(t)}\frac{P_t^2(ij)}{Q_t(ij)}\right)-2p_{t-1}(i)+q_{t-1}(i)\\
%=\frac{p_{t-1}^2(i)}{q_{t-1}(i)}\sum_{j:(ij)\in E(t)}\left(\frac{\left(P_t(ij)-Q_t(ij)\right)^2}{Q_t(ij)}+
%2P_t(ij)-Q_t(ij)\right)-2p_{t-1}(i)+q_{t-1}(i)\\
=\frac{p_{t-1}^2(i)}{q_{t-1}(i)}\sum_{j:(ij)\in E(t)}\frac{\left(P_t(ij)-Q_t(ij)\right)^2}{Q_t(ij)}+
\frac{\left(p_{t-1}(i)-q_{t-1}(i)\right)^2}{q_{t-1}(i)}\\
%= \frac{p_{t-1}^2(i)}{q_{t-1}(i)}\sum_{j:(ij)\in E(t)}\left(\sqrt{P_t(ij)}-\sqrt{Q_t(ij)}\right)^2\left(\frac{\sqrt{P_t(ij)}+\sqrt{Q_t(ij)}}{\sqrt{Q_t(ij)}}\right)^2+
%\frac{\left(p_{t-1}(i)-q_{t-1}(i)\right)^2}{q_{t-1}(i)}\\
\ge \frac{p_{t-1}^2(i)}{q_{t-1}(i)}\sum_{j:(ij)\in E(t)}\left(\sqrt{P_t(ij)}-\sqrt{Q_t(ij)}\right)^2+\frac{\left(p_{t-1}(i)-q_{t-1}(i)\right)^2}{q_{t-1}(i)},
\label{eq:inequality_sqrtpq}
\end{multline}
where the third and forth equalities hold true as $\sum_{j:(ij)\in E(t)}P_t(ij)=\sum_{j:(ij)\in E(t)}Q_t(ij)=1$, and to get the last inequality one can simply use identity 
$\frac{(a-b)^2}{b}=(\sqrt{a}-\sqrt{b})^2\left(\frac{\sqrt{a}+\sqrt{b}}{\sqrt{b}}\right)^2$. Now, we claim that the expression in RHS of \eqref{eq:inequality_sqrtpq} is 
at least RHS of \eqref{eq:dist_sqrtpq} for a given $i$, i.e., we need to show that
\be
\label{eq:inequality_four_deg_poly}
\left(\frac{p_{t-1}^2(i)}{q_{t-1}(i)}-\frac{\sqrt{p_{t-1}(i)q_{t-1}(i)}}{2}\right)\sum_{j:(ij)\in E(t)}\left(\sqrt{P_t(ij)}-
\sqrt{Q_t(ij)}\right)^2+\frac{\left(p_{t-1}(i)-q_{t-1}(i)\right)^2}{q_{t-1}(i)}\ge 0.
\ee
The inequality is obviously true, if $\frac{p_{t-1}^2(i)}{q_{t-1}(i)}\ge\frac{\sqrt{p_{t-1}(i)q_{t-1}(i)}}{2}$.
Otherwise, without loss of generality, we can substitute the term 
\[
\sum_{j:(ij)\in E(t)}\left(\sqrt{P_t(ij)}-\sqrt{Q_t(ij)}\right)^2
\] 
with an upper bound of $2$. Furthermore, by denoting $x=\sqrt{\frac{p_{t-1}(i)}{q_{t-1}(i)}}$ the inequality \eqref{eq:inequality_four_deg_poly} can be rewritten as
$q_{t-1}(i)\cdot\left(2x^4-x+(x^2-1)^2\right)\ge 0$, and, indeed, one can verify that this fourth degree polynomial is always positive.
\end{proof}

Now we estimate the variance of random variable $Z$

\begin{lemma}
$\Ex{Z}\ge \left(\frac{12\sqrt{2k}}{C}+\frac{2\sqrt{2}+\sqrt{k}}{\sqrt{C}}\right)\cdot\sqrt{\Var{Z}}$, when $m\ge \frac{C\cdot n^{3/2}}{\eps^2}$ and $\dist{P}{Q}\ge \eps$.
\label{cl:var_z}
\end{lemma}
\begin{proof}
We recall that $Z=\sum_{e\in E}Z_e$ and by Lemma~\ref{cl:ind_poisson} all $Z_e$ for a fixed $t$ and $e\in E(t)$ are independent.
For any random variables $X_1,\dots, X_n$ it is true that 
\[
\Var{X_1+\cdots+X_n}\le\left(\sqrt{\Var{X_1}}+\cdots+\sqrt{\Var{X_n}}\right)^2.
\]
We use this estimate for $X_t=\sum_{e\in E(t)}Z_e$ to obtain
\[
\sqrt{\Var{Z}}\le\sum_{t=1}^n\sqrt{\sum_{e\in E(t)}\Var{Z_e}}=\sum_{t=1}^n\sqrt{\sum_{e\in E(t)}2\frac{p_e^2}{q_e^2}+m\cdot\frac{p_e(p_e-q_e)^2}{q_e^2}}
\]
We further simplify the above expression by using the fact that $\sqrt{x+y}\le \sqrt{x}+\sqrt{y}$.
\be
\sqrt{\Var{Z}}\le\sum_{t=1}^n\sqrt{\sum_{e\in E(t)}2\frac{p_e^2}{q_e^2}}+\sqrt{m}\sum_{t=1}^n\sqrt{\sum_{e\in E(t)}\frac{p_e(p_e-q_e)^2}{q_e^2}}
\label{eq:var_sqrt_ub}
\ee

On the other hand, by Lemma~\ref{cl:expectation_dist}
\be
\label{eq:expectation_def_eps}
\Ex{Z}\ge \frac{1}{2}\Ex{Z} + \frac{m}{8}\distsq{P}{Q} =  m\cdot\left(\frac{1}{2}\sum_{e\in E}\frac{(p_e-q_e)^2}{q_e}+\frac{\eps^2}{8}\right).
\ee
In the following we use \eqref{eq:expectation_def_eps} to give separate upper bounds on each of the two summation terms in the 
RHS of \eqref{eq:var_sqrt_ub}. 

\paragraph{First term of \eqref{eq:var_sqrt_ub}.} To estimate the first term, we split $E$ into two sets 
\[
E_1\eqdef\{e\in E: p_e\le 2q_e\} \quad\text{and}\quad E_2\eqdef\{e\in E: p_e> 2q_e\}
\]
We define accordingly the sets $E_1(t)$ and $E_2(t)$ for each $t\in[n]$. Again we have
\beq
\sum_{t=1}^n\sqrt{\sum_{e\in E(t)}2\frac{p_e^2}{q_e^2}}\le \sum_{t=1}^n\sqrt{\sum_{e\in E_1(t)}2\frac{p_e^2}{q_e^2}} + \sum_{t=1}^n\sqrt{\sum_{e\in E_2(t)}2\frac{p_e^2}{q_e^2}}.
\eeq
\textbf{Estimate for $\mathbf{E_1}$.} 
We have $2\frac{p_e^2}{q_e^2}\le 8$ for any edge $e\in E_1$. Therefore, by the sparsity condition $\sum_{e\in E_1(t)}2\frac{p_e^2}{q_e^2}\le 8n\cdot k$, where $k=O(1)$.
Thus, 
%\nick{determine $c_1$}
\be
\sum_{t=1}^n\sqrt{\sum_{e\in E_1(t)}2\frac{p_e^2}{q_e^2}}\le \sqrt{8k}\cdot n^{3/2}\le \frac{\sqrt{8k}}{C} \cdot m\cdot \eps^2 \le \frac{4\sqrt{8k}}{C}\cdot\Ex{Z} 
\label{eq:e1}
\ee
\textbf{Estimate for $\mathbf{E_2}$.} We have $\frac{(p_e-q_e)^2}{q_e}\ge \frac{p_e^2}{4q_e}$ for any $e\in E_2$. Therefore,
%\nick{$c_2\cdot m\frac{\eps^2}{4n^{3/2}}=1$}
\begin{multline}
\frac{\sqrt{32k}}{C}\cdot\Ex{Z}\ge \frac{\sqrt{32k}m}{C}\cdot\sum_{t=1}^n\left(\frac{1}{16}\sum_{e\in E_2(t)}2\frac{p_e^2}{q_e}+\frac{\eps^2}{8n}\right)
\ge \frac{\sqrt{32k}m}{C}\sqrt{\frac{4\eps^2}{16\cdot 8n}}\sum_{t=1}^n \sqrt{\sum_{e\in E_2(t)}2\frac{p_e^2}{q_e}}\\
\ge \frac{\sqrt{32k}m}{C}\sqrt{\frac{\eps^2}{32n}}\cdot\sqrt{\frac{\eps^2}{kn^2}}\sum_{t=1}^n \sqrt{\sum_{e\in E_2(t)}2\frac{p_e^2}{q_e^2}}
\ge \sum_{t=1}^n \sqrt{\sum_{e\in E_2(t)}2\frac{p_e^2}{q_e^2}},
\label{eq:e2}
\end{multline}
where the first inequality holds by \eqref{eq:expectation_def_eps}; the second inequality is simply AM-GM inequality; and to get the third
inequality we used the bound $q_e\ge\frac{\eps^2}{kn^2}$.

\paragraph{Second term  of \eqref{eq:var_sqrt_ub}.} We split $E$ into another two sets $E_3,E_4$ (similarly define $E_3(t)$ and $E_4(t)$): 
\[
E_3\eqdef\{e\in E: p_e\le 2\sqrt{n}q_e\} \quad\text{and}\quad E_4\eqdef\{e\in E: p_e> 2\sqrt{n}q_e\}
\]
\[
\text{Again}\quad \sum_{t=1}^n\sqrt{\sum_{e\in E(t)}\frac{p_e(p_e-q_e)^2}{q_e^2}}\le\sum_{t=1}^n\sqrt{\sum_{e\in E_3(t)}\frac{p_e(p_e-q_e)^2}{q_e^2}}+
\sum_{t=1}^n\sqrt{\sum_{e\in E_4(t)}\frac{p_e(p_e-q_e)^2}{q_e^2}}
\]
\textbf{Estimate for $\mathbf{E_3}$.} We have 
\begin{multline}
2\sqrt{\frac{2}{C}}\cdot\Ex{Z}\ge \sqrt{\frac{2}{C}}m\cdot\sum_{t=1}^n\left(\sum_{e\in E_3(t)}\frac{(p_e-q_e)^2}{q_e}+\frac{\eps^2}{4n}\right)\ge
\sqrt{\frac{2}{C}}m\sqrt{\frac{\eps^2}{n}}\sum_{t=1}^n\sqrt{\sum_{e\in E_3(t)}\frac{(p_e-q_e)^2}{q_e}}\\
\ge m\sqrt{\frac{2\eps^2}{Cn}}\cdot \sqrt{\frac{1}{2n^{1/2}}}\sum_{t=1}^n\sqrt{\sum_{e\in E_3(t)}\frac{p_e(p_e-q_e)^2}{q_e^2}}
= \sqrt{m}\sum_{t=1}^n\sqrt{\sum_{e\in E_3(t)}\frac{p_e(p_e-q_e)^2}{q_e^2}},
\label{eq:e3}
\end{multline}
where the first inequality holds by \eqref{eq:expectation_def_eps}, the second inequality is AM-GM inequality, to get the third inequality
we use definition of $E_3$ that $\frac{p_e}{q_e}\le 2\sqrt{n}$.\newline
\textbf{Estimate for $\mathbf{E_4}$.} We have $p_e-q_e\ge \left(1-\frac{1}{2\sqrt{n}}\right)p_e$ for any $e\in E_4$. Therefore,
\begin{multline}
\frac{\sqrt{k}}{\sqrt{2C}\left(1-\frac{1}{2\sqrt{n}}\right)}\cdot\Ex{Z}\ge \frac{m\sqrt{k}}{\sqrt{2C}}\sum_{e\in E_4}\frac{p_e(p_e-q_e)}{q_e}\ge
\sqrt{m}\sqrt{\frac{km\cdot2\eps^2 }{2C\cdot kn^{3/2}}}\sum_{e\in E_4}\frac{p_e^{1/2}(p_e-q_e)}{q_e}\\
\ge\sqrt{m}\sum_{t=1}^n\sqrt{\sum_{e\in E_4(t)}\frac{p_e^{1/2}(p_e-q_e)}{q_e}},
\label{eq:e4}
\end{multline}
where the first inequality follows from\eqref{eq:expectation_def_eps}, to get the second inequality we estimate $\sqrt{p_e}\ge \sqrt{2n^{1/2}q_e}\ge\sqrt{\frac{2\eps^2}{kn^{3/2}}},$
to get the last inequality we simply use that $\sqrt{x}+\sqrt{y}\ge\sqrt{x+y}$. 

Finally, combining estimates \eqref{eq:e1},\eqref{eq:e2},\eqref{eq:e3},\eqref{eq:e4} we obtain the desired bound on the variance.
\end{proof}

\begin{lemma}
If $P=Q$, then $\Var{Z}\le\sqrt{k}n^{3/2}$.
\label{cl:var_z_easy}
\end{lemma}
\begin{proof}
Using similar estimate as in the proof of Lemma~\ref{cl:var_z} we get
\[
\sqrt{\Var{Z}}\le\sum_{t=1}^n\sqrt{\sum_{e\in E(t)}\Var{Z_e}}=\sum_{t=1}^n\sqrt{\sum_{e\in E(t)}2\frac{q_e^2}{q_e^2}}\le n\cdot\sqrt{kn}.
\]
\end{proof}

To conclude the proof of Theorem~\ref{th:sparse_ub} it remains to notice that in case $P=Q$ the error probability (Algorithm~\ref{alg:chi_sq_edges} returns ``reject'') is at most
\[
\Prx{Z> 2\sqrt{k}n^{3/2}}\le\Prx{Z> 2\sqrt{\Var{Z}}}\le \frac{1}{5},
\]
where the first inequality follows from Lemma~\ref{cl:var_z_easy}, the last is Cantelli's inequality, since $\Ex{Z}=0$.
On the other hand, when $\dist{P}{Q}\ge \eps$, then $\Ex{Z}\ge m\cdot\frac{\eps^2}{4}$. If Algorithm~\ref{alg:chi_sq_edges} makes an error by returning ``accept'', 
then $Z\le 2\sqrt{k}n^{3/2}\le \frac{2\sqrt{k}}{C}\Ex{Z}$. Thus $Z-\Ex{Z}\le (\frac{2\sqrt{k}}{C}-1)\Ex{Z}$. Now if $C$ is such that
$1-\frac{2\sqrt{k}}{C}\ge 2\cdot\left(\frac{12\sqrt{2k}}{C}+\frac{2\sqrt{2}+\sqrt{k}}{\sqrt{C}}\right)$ (any constant 
$C\ge\max\left(\sqrt{k}(42\sqrt{2}+4),(8\sqrt{2}+4\sqrt{k})^2\right)$ would work), then $Z-\Ex{Z}\le -2\sqrt{\Var{Z}}$ by Lemma~\ref{cl:var_z}. Furthermore,
by Cantelli's inequality 
\[
\Prx{Z\le 2\sqrt{k}n^{3/2}}\le \Prx{Z-\Ex{Z}\le -2\sqrt{\Var{Z}}}\le \frac{1}{5},
\]
i.e., probability of Algorithm~\ref{alg:chi_sq_edges}'s error in the case $P\neq Q$ is at most $\frac{1}{5}$.  
\end{proof}

\paragraph{Analysis of pruning step.} Here we slightly modify Markov Chains $Q$ and $P$ so that probability of traversing any edge in $Q$ is $\Omega(\frac{\eps^2}{n^2})$ and that 
$P$ only uses these edges. To this end, we sequentially remove edges from $Q$ that have too low probability of traversal in $Q$. Effectively, in the pruning process we are sampling from $Q$, but rejecting all the 
samples that use a ``rare'' edge. We choose the threshold for the ``rare'' edges in such a way that we would reject at most $\eps^2$ fraction of samples from $Q$. Recall that the Markov chain obtained by pruning $Q$ is denoted as $Q^*$.
After pruning of $Q$, we do the corresponding empirical rejection sampling for $P$ (see Algorithm~\ref{alg:pruning}) which is equivalent to obtaining samples from the modified Markov chain $P^*$. If there are too many rejected samples, 
we conclude that $\dist{P}{P^*}>\dist{Q}{Q^*}$ with high probability, and thus $P\neq Q$. Otherwise we proceed to Algorithm~\ref{alg:chi_sq_edges} for the modified $Q$ and pruned samples 
from $P$. 

\begin{algorithm}%[H]
\caption{Pruning Test. In the pruned Markov Chain $Q^*$ all edges with $q_e>0$ satisfy $q_e\ge\frac{\eps^2}{kn^2};$ samples from Markov Chain $P^*$ can only go along these edges.}
\label{alg:pruning}
\SetKwData{Recompute}{Recompute}\SetKwData{Samples}{PrunedSamples}\SetKwData{Count}{RejectCount}
\SetKwFunction{Delete}{Delete}
\KwIn{$\eps$; an explicit $k$-sparse Markov Chain $Q=\MCseqQ$; $m$ samples from a Markov Chain $P=\MCseqP$}
\KwOut{$m\cdot(1-2\eps^2)$ i.i.d. samples from pruned $P^*$ and pruned $Q^*$ s.t., each $q_e=\Omega(\frac{\eps^2}{n^2})$; reject $P$ if there are not enough samples.}
\BlankLine
Let $E^*=\{e: q_e>0\}$\;
\While{$\exists~e\in E^*:q_{e}<\frac{\eps^2}{k\cdot n^2}$}{
$E^*\leftarrow E^*\setminus e$\tcc*{$e=(ij)$, $e\in E(t)$}
\Delete($e,Q$)\tcc*{set $Q_t(ij)=0$, re-normalize row $i$ in $Q_t$}
\lForEach{edge $e\in E^*$}{\Recompute{$q_e$}}
}
\For{$w=s_1\cdots s_n \sim P$}{
\lIf{$\forall~t~ (s_ts_{t+1})\in E^*$}{Add $w$ to \Samples}
\lElse{increase \Count}
}
\eIf{\Count$>2m\eps^2$}
{
\KwRet \textsc{Reject}\;  
}
{
\KwRet \Samples\;  
}
\end{algorithm}

Let $Q^*$ be a modified Markov Chain $Q$ that sample $w\sim Q$ and reject any $w$ with $e\notin E^*$.
\begin{lemma}
$\dist{Q}{Q^*}\le 2\eps^2$
\label{cl:rejection_Q}
\end{lemma}   
\begin{proof}
By definition of the set of pruned edges $E^*$, by removing each new edge we lose at most $\frac{\eps^2}{kn^2}$ fraction of samples.
As there are only at most $kn^2$ edges in $Q$, the probability of avoiding removed edges is at least
$(1-\frac{\eps^2}{kn^2})^{kn^2}\ge 1-\eps^2$. Thus at most $\eps^2$ fraction of words $\word{Q}{n}$ are rejected in $\word{Q^*}{n}$, which implies that
$2\eps^2\le\dtv{\word{Q}{n}}{\word{Q^*}{n}}=\dist{Q}{Q^*}$.
\end{proof}

We need to argue about probability of error in Algorithm~\ref{alg:pruning}. First, in the case $P=Q$ Algorithm~\ref{alg:pruning} could incorrectly return ``reject''.
Our next Lemma~\ref{cl:error_prob_pruning} provides the necessary bound. On the other hand, when $P\neq Q$ and  Algorithm~\ref{alg:pruning} does not return ``reject'', we 
want Algorithm~\ref{alg:chi_sq_edges} to be able to distinguish $P^*$ and $Q^*$. To this end, Lemma~\ref{cl:error_prob_pruning} shows that $\dist{P^*}{Q^*}=\Omega(\eps)$ 
with high probability.

%Therefore, in the case $P=Q$ we have $\dist{P}{P^*}\le 2\eps^2$. In this case we show that Algorithm~\ref{alg:pruning} does not reject $P$
%with high probability. On the other hand, if $P\neq Q$ and Algorithm~\ref{alg:pruning} does not reject $P$, 
%we want to make sure that Algorithm~\ref{alg:chi_sq_edges} will distinguish $P^*$ and $Q^*$. To this end, we need to provide a lower bound on 
%$\dist{P^*}{Q^*}\ge\eps-\dist{P}{P^*}-\dist{Q}{Q^*}$. As $\dist{Q}{Q^*}\le 2\eps^2$, for a lower bound of $\dist{P^*}{Q^*}\ge\frac{\eps}{4}$ 
%it would suffice to show that $\dist{P^*}{P}\le\frac{\eps}{2}$.
\begin{lemma}~
\label{cl:error_prob_pruning}

(1) If $P=Q$, then Algorithm~\ref{alg:pruning}'s error of rejecting $P$ is at most $0.1$.

(2) If $\dist{P}{Q}\ge \eps$, then either $\dist{P^*}{Q^*}=\Omega(\eps)$, or Algorithm~\ref{alg:pruning} correctly rejects $P$ with probability at least $0.9$.
\end{lemma}
\begin{proof}
Let $X_\ell$ be Bernoulli random variables for $\ell\in[m]$ denoting ($X_\ell=1$) whether $\ell$-th sample from $P$ was rejected, or accepted to $P^*$ ($X_\ell=0$).  
Then the number of rejected samples $X=\sum_{\ell=1}^m X_\ell$. Variables $X_\ell$ are i.i.d. Let $x=\Prx{X=1}$.

1. If $P=Q$, then probability of rejecting a sample from $P$ is not more than $\eps^2$, i.e., $x\le \eps^2$. $\Ex{X}=m\cdot x, \Var{X}=m\cdot(x-x^2)$. Then
\[
\Prx{X\ge 2m\eps^2}\le\Prx{X\ge \Ex{X}+3\sqrt{\Var{X}}}\le\frac{1}{10},
\]
where the first inequality holds because $2m\eps^2> m\cdot \eps^2 + 3\sqrt{m\eps^2}>\Ex{X}+3\sqrt{\Var{X}}$; the second is Cantelli's inequality.

2. We first observe that $\dist{P^*}{Q^*}\ge\eps-\dist{Q}{Q^*}-\dist{P}{P^*}$. We want to argue that if $\dist{P}{P^*}\ge 6\eps^2$, then
Algorithm~\ref{alg:pruning} rejects $P$ with probability at least $9/10$. Indeed, then probability $x$ of rejecting a sample from $P$ must be at least 
$\frac{1}{2}\dist{P}{P^*}\ge 3\eps^2$, then $\Ex{X}\ge 3m\eps^2$ and
\[
\Prx{X\le 2m\eps^2}\le\Prx{X-\Ex{X}\le -\frac{\Ex{X}}{3}}\le\Prx{X-\Ex{X}\le -3\sqrt{\Var{X}}}\le\frac{1}{10}.
\]
Thus we get $\dist{P^*}{Q^*}\ge\eps-\dist{Q}{Q^*}-\dist{P}{P^*}\ge\eps-2\eps^2-6\eps^2\ge\frac{\eps}{2}$ if $\eps$ is small enough constant. 
\end{proof}

\begin{theorem}
Together, Algorithm~\ref{alg:pruning} and Algorithm~\ref{alg:chi_sq_edges} tell whether $P=Q$, 
or $P\neq Q$, when $\dist{P}{Q}\ge\eps$,  with probability at least $\frac{2}{3}$ using $O(\frac{n^{3/2}}{\eps^2})$ samples.
%\label{th:main_shuffling}
\end{theorem}
\begin{proof}
In case $P=Q$, Algorithm~\ref{alg:pruning} produces $P^*=Q^*$ and $m(1-2\eps^2)$ samples from $P^*$ with probability at least $0.9$.
Furthermore, Algorithm~\ref{alg:chi_sq_edges} converts these $m(1-2\eps^2)$ samples into Poisson $m'=\Omega(m)$ samples and accepts
$P=Q$ with $4/5$ probability. Overall, we have $4/5\cdot 0.9>2/3$ probability of correctly accepting $P=Q$.

When $\dist{P}{Q}\ge\eps$, Algorithm~\ref{alg:pruning} either correctly rejects $P^*$, or produces $P^*$ and $Q^*$ s.t. $\dist{P^*}{Q^*}\ge\frac{\eps}{2}$ with probability at least $0.9$. In the latter case Algorithm~\ref{alg:chi_sq_edges} correctly rejects $P^*$ with probability at least $4/5$. Overall, we get the probability of correctly rejecting $P$ to be at least $4/5\cdot 0.9>2/3$.
\end{proof}
